# Supplementary material for: Re4: Learning to Re-contrast, Re-attend, Re-construct for Multi-interest Recommendation
Source: arXiv:2208.08011 source file (2024-02-21)
Supplement: Supplementary file 1 [file 6.Appendix.tex]

\section{Appendix}
\label{sec:appendix}
